# Supplementary material for: Inclusive Search for Anomalous Single-Photon Production in MicroBooNE
Source: arXiv:2502.06064 ancillary file (2026-10-15)
Supplement: Supplementary file 1 [file supp_uB_inclusive_single_photon_LEE_PRL_journal_submit.pdf]

# Supplemental Material: Inclusive Search for Anomalous Single-Photon Production in MicroBooNE

## I. INTRODUCTION

In this Supplemental Material, we provide further information on the inclusive single-photon selected events and surrounding analysis. This includes information about the systematic errors and efficiencies of the main selection, the BDT score distributions used for the selections, distributions for the constraining channels used in statistical tests for both the initial result and the zero-proton ROI, further information on the MiniBooNE photon-like LEE (“LEE- $\gamma$ ”) model, and kinematic distributions for single-photon events with shower energies between 0 and 600 MeV with 1 or more protons.

## II. SELECTION: EFFICIENCIES AND SYSTEMATICS

Figure. 1 shows the split between different sources of systematic uncertainty on the  $1\gamma$  signal channel and the two sideband constraint channels with NC  $\pi^0$  and  $\nu_\mu$  CC event topologies. The plot shows the percentage split across the sources of systematic uncertainty considered in the analysis: flux, cross sections (“XS”), detector, Monte Carlo statistics, and “dirt” systematic uncertainty associated with interactions occurring outside of the cryostat volume. More information on these uncertainty sources and how they are incorporated and considered in this analysis can be found in Ref. [1].

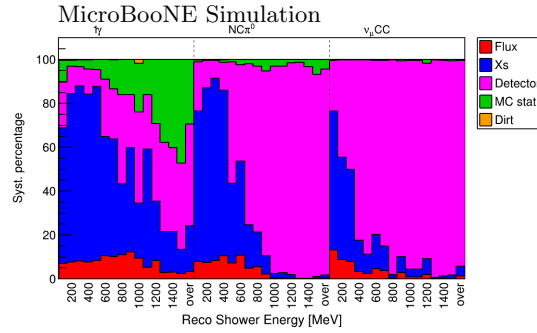

FIG. 1. Summary of fractional contributions to the overall systematic uncertainty ( $(\sigma_i^2/\sigma_{\text{total}}^2) \times 100$ ), before constraint, for the signal (left) and two constraining channels, with the NC  $\pi^0$  channel in the center and the  $\nu_\mu$  CC channel on the right.

Figure 2 shows the signal selection efficiency as a function of the photon shower energy and angle. The efficiency is fairly flat as a function of shower angle, and rises smoothly with shower energy.

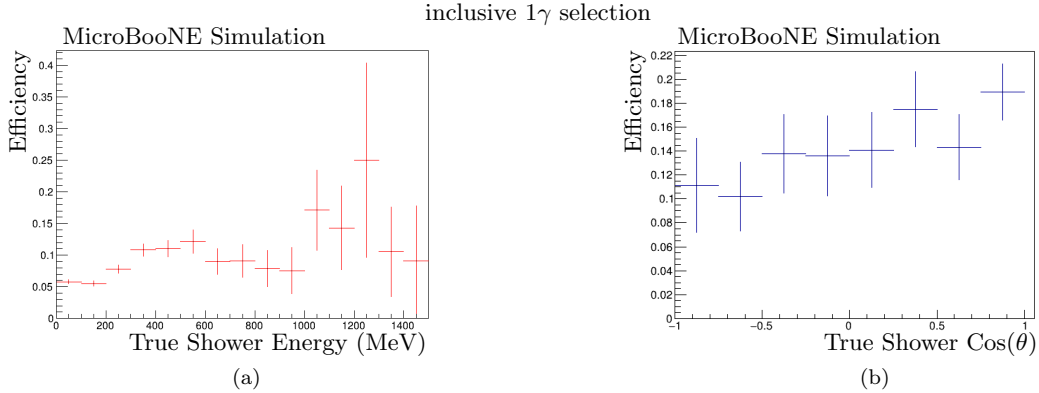

FIG. 2. The efficiency of the single-photon signal sample as a function of true shower energy (a) and cosine of the true angle with respect to the beam direction (b).

### III. BDT SCORES

The selection is applied using a series of four BDTs, the distributions for three of which are shown in Figure 3. The fourth BDT — aimed at separating single-photon and single-electron events — is shown in the main text. The BDT cut values are chosen using a simultaneous optimization method. The metric  $E \times P^2$ , where  $E$  is the signal efficiency and  $P$  is the signal purity, is calculated at every point in a  $4 \times 4$  grid of the BDT scores. The grid point with the maximum value is then found and the BDT scores corresponding to that point are used as the cut values for the selection.

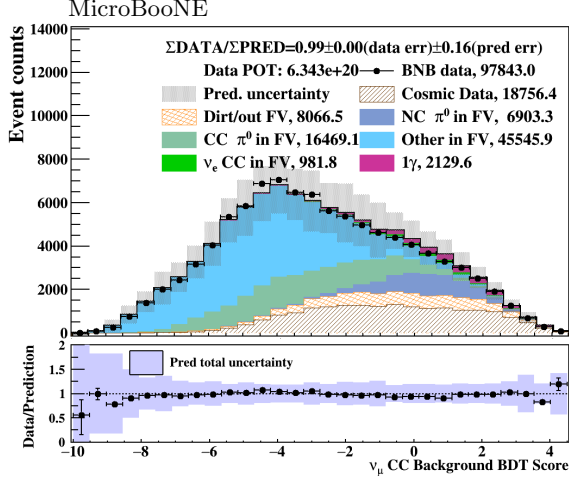

(a)  $\nu_\mu$  CC BDT score for events that have passed preselection. Events with values greater than 0.4 are considered signal-like and go forward to the next (Other) BDT. Events with values less than 0.1 are used for the  $\nu_\mu$  CC sideband and constraint sample.

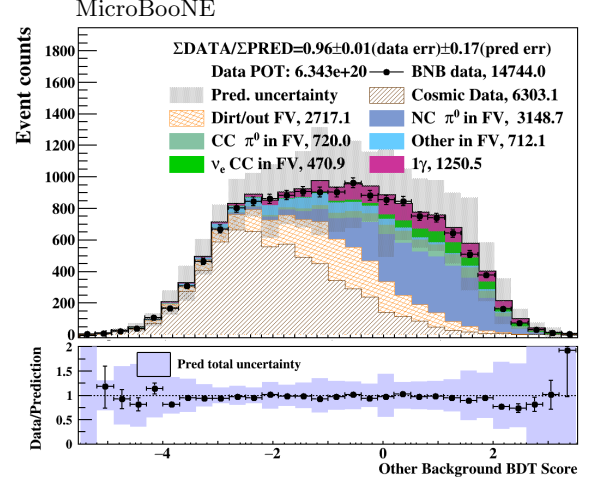

(b) Other BDT score for events that have passed preselection and the  $\nu_\mu$  CC BDT. Events with values greater than 0.2 are considered signal-like and go forward to the next (NC  $\pi^0$ ) BDT. Events with values less than -0.4 are used for the Other sideband, which is used only for validation and not constraints.

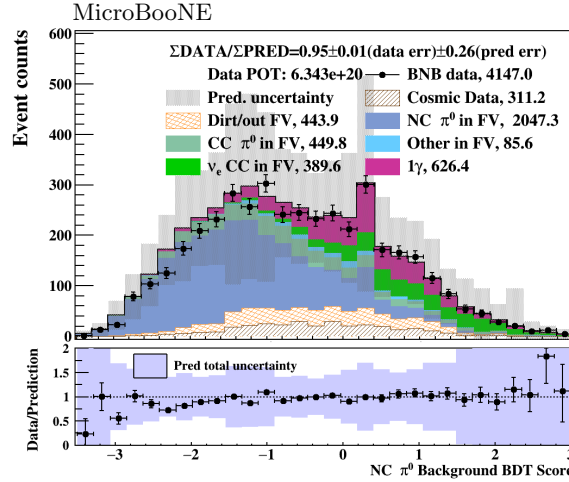

(c) NC  $\pi^0$  BDT score for events that have passed preselection and the previous BDTs. Events with values greater than -0.05 are considered signal-like and go forward to the next ( $\nu_e$  CC) BDT. Events with values less than -0.4 are used for the NC  $\pi^0$  sideband and constraint sample.

FIG. 3. BDT score distributions for three of the four BDTs used in the selection. The fourth ( $\nu_e$  CC) is shown in the main text of the paper. Pink shows the signal  $1\gamma$  events.

#### IV. SIDEBAND CONSTRAINT

This section shows the distribution of selected events in the channels used to constrain the signal and background prediction in the signal region. Figure 4 shows the NC  $\pi^0$  and  $\nu_\mu$  CC selected event distributions as a function of reconstructed shower energy. Both show good agreement within systematic uncertainties. Figure 5 shows the correlation matrix between the signal region and these sidebands used in the constraint procedure. We see a very strong correlation between events in the NC  $\pi^0$  sideband and signal channel at energies below 600 MeV, which is a consequence of the large contribution of true NC  $\pi^0$  events in the signal sample. Further details on the constraint procedure can be found in Ref. [1].

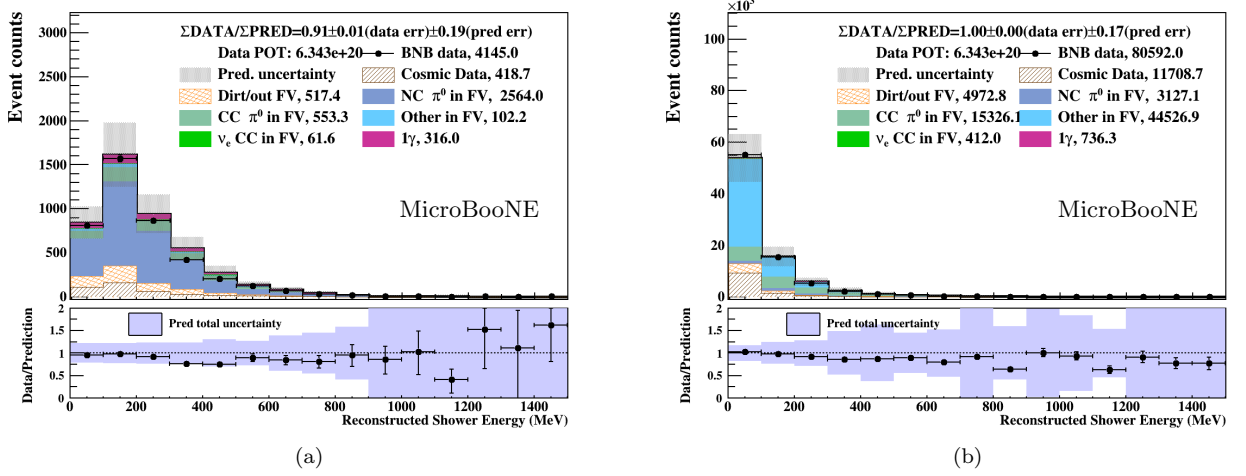

FIG. 4. Reconstructed shower energy for the NC  $\pi^0$  (a) and  $\nu_\mu$  CC (b) sidebands used for constraining the signal channel.

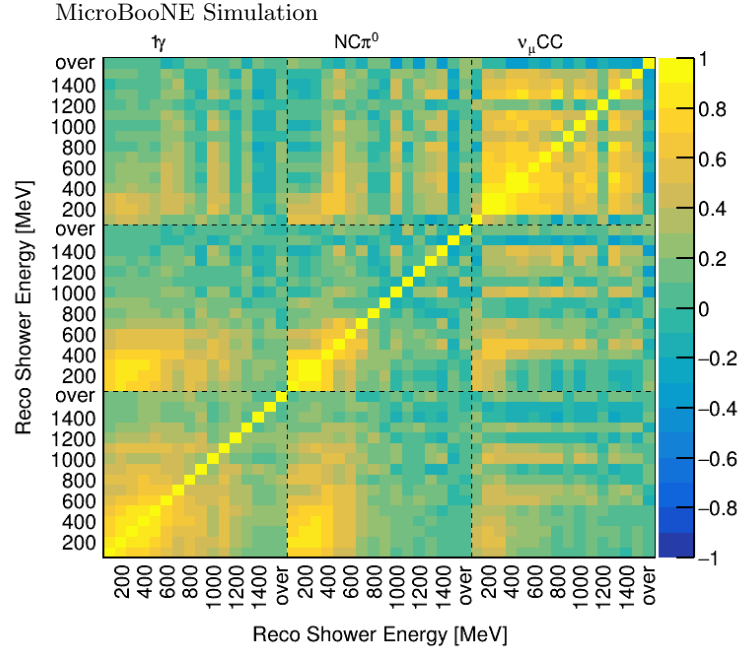

FIG. 5. Correlation matrix between constraint sidebands and signal region.

Figure 6 shows the same two sideband channels but for the 0p sub-sample. These distributions are used to constrain

the  $1\gamma 0p$  ROI signal channel.

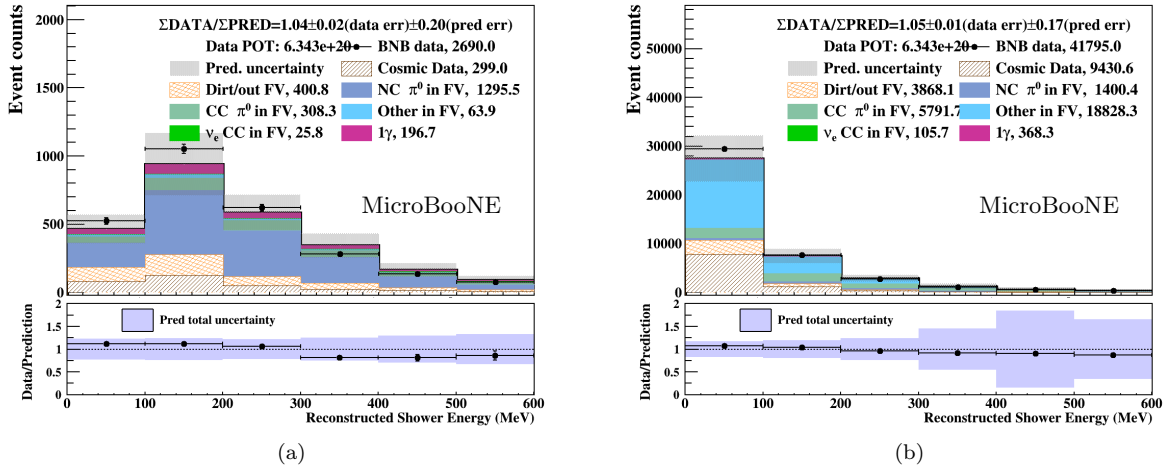

FIG. 6. Reconstructed shower energy for the NC  $\pi^0$  (a) and  $\nu_\mu$  CC (b) sidebands with no protons above the 35 MeV proton reconstructed kinetic energy threshold used for constraining the zero-proton signal channel.

## V. SIGNAL KINEMATICS DISTRIBUTIONS

Figures 7, 8, and 9 show the distributions of the  $1\gamma$  signal channel (the full Xp distribution, as well as the exclusive  $1\gamma 0p$  ROI sub-sample) in various kinematic variables of interest. Plots shown include the data-simulation comparison where predictions are split in signal and background categories, as well as a comparison of data to the pre- and post-constraint prediction, shown in red and blue, respectively. The quantitative goodness-of-fit via a  $\chi^2/n.d.f.$  metric of each distribution is also shown.

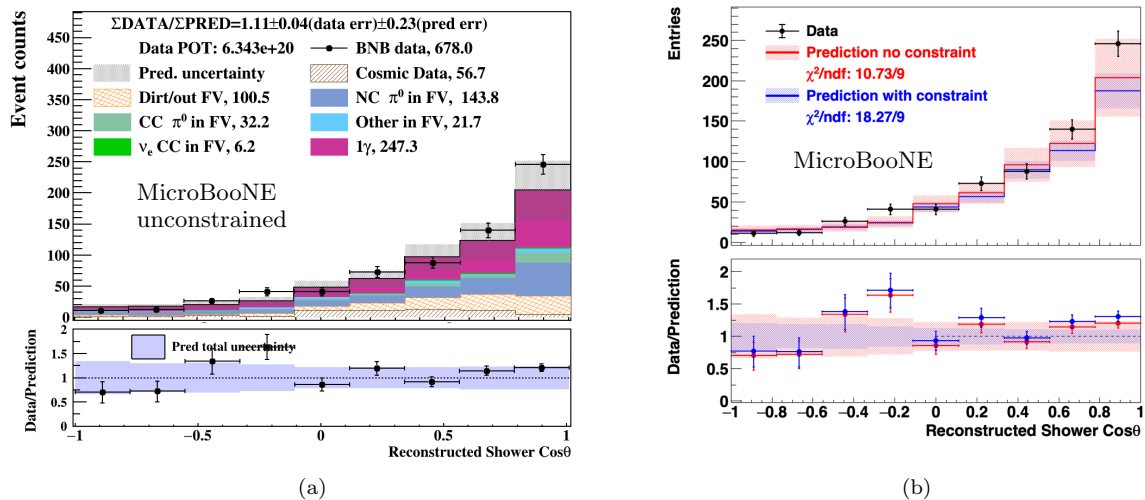

FIG. 7. (a): Cosine of reconstructed shower angle with respect to the beam for inclusive single-photon selected events. The solid pink shows the inclusive single-photon signal events. A slight (11%) data excess, concentrated in the two most forward-going (0.6–1.0) bins, is observed but within the uncertainties. (b): Cosine of reconstructed shower angle with respect to the beam direction for inclusive single-photon selected events, before and after constraint. The horizontal axis is reconstructed shower angle with bin size of  $\sim 0.22$ .

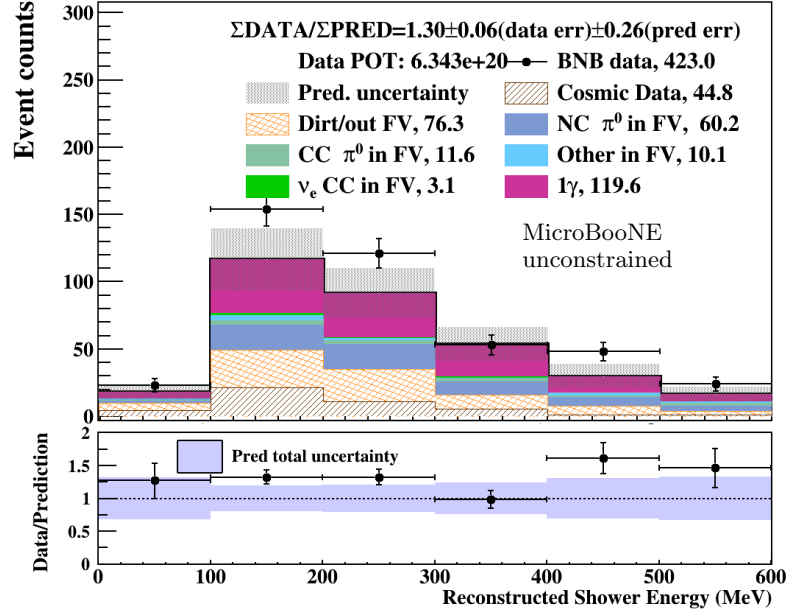

FIG. 8. Reconstructed shower energy for exclusive  $1\gamma 0p$  selected events, before constraint. The solid pink shows the signal events.

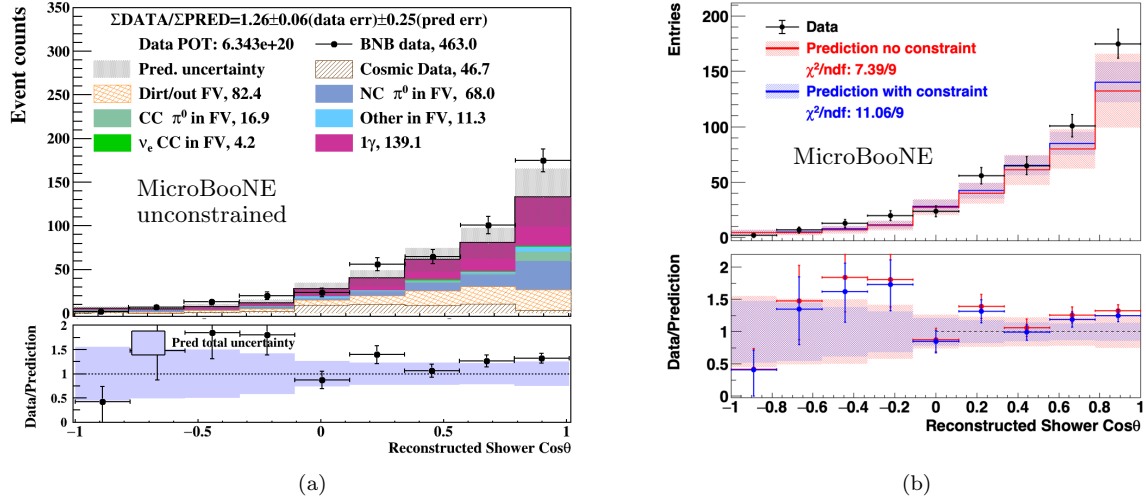

FIG. 9. (a): Cosine of reconstructed shower angle with respect to the beam for the exclusive  $1\gamma 0p$  selected events. Signal is shown in solid pink. (b): Cosine of reconstructed shower angle with respect to the beam for the exclusive  $1\gamma 0p$  selected events, before (red) and after (blue) constraint. The horizontal axis is reconstructed shower angle with bin size of  $\sim 0.22$ .

Figure 10 shows the backwards projected distance to the nearest TPC wall, which is measured as the distance to the nearest TPC boundary in the direction opposite that of the reconstructed shower direction, for the  $0p$  signal sample. This variable is intended to help provide shape information that can discriminate between photons originating from neutrino interactions occurring inside versus outside of the TPC volume, and therefore helps investigate the possible mis-modeling of different contributions such as Dirt or other out-of-FV backgrounds. While single-photon events with no reconstructed protons are identified in the detector's fiducial volume, the relatively large conversion distance for photons in argon makes it possible that such events originate from interactions which occur outside of the TPC FV. Furthermore, the elongated shape of the MicroBooNE experiment makes it so that any portion of the detector volume is relatively close to a detector edge. These two features inevitably lead to a relatively large probability of

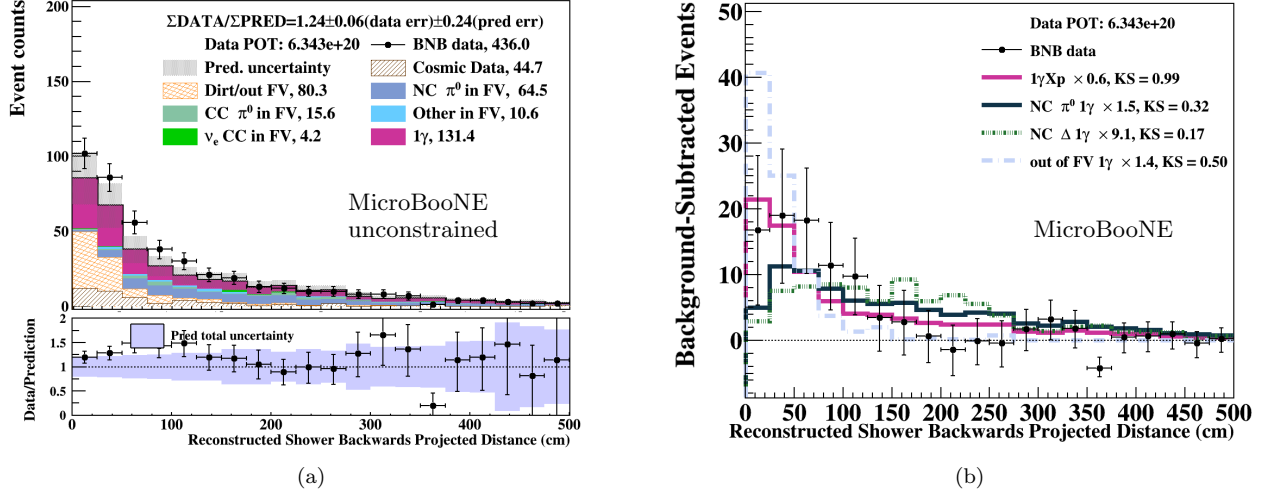

FIG. 10. Reconstructed shower backward projected distance for the  $1\gamma 0p$  subsample. This measures the distance from the shower start to the closest TPC wall when tracing backwards along the shower trajectory. For reference, the detector is 2.5 m long in the drift direction, 2.3 m in vertical direction, and 10.4 m long in the beam direction. (a) shows the Data-MC comparison distribution for this variable, with inclusive single-photon signal events in solid pink. (b) shows a shape-only fit for  $1\gamma 0p$  background-subtracted events (data minus prediction) for this variable. Three signal categories, as well as the total “ $1\gamma Xp$ ” signal, are shown alongside the best fit scaling parameter and the Kolmogorov-Smirnov test statistic. We do not apply a sideband constraint to the excess predictions. The error bars on the data points include both statistical and constrained systematic errors.

selecting events that have a true origin outside of the detector. The distribution of Figure 10 shows this. The first few bins (below 50 cm) are heavily contaminated by Dirt and Out-of-FV events. NC  $\pi^0$  events in blue, on the other hand, populate the distribution more uniformly. Predicted  $1\gamma$  signal events in solid pink consist of a mix of photons which originate from interactions outside and inside the TPC FV. Additionally, a shape-only fit to  $1\gamma 0p$  background-subtracted (“excess”) events, using the same framework as Figure 5 in the main body of the paper, is shown for this distribution for the three signal categories with the highest KS score, as well as the total  $1\gamma$  signal. It can be seen from the KS score numbers that the total signal category of all inclusive single-photon events fits the shape of this distribution (at a KS score of 0.99) better than any single signal category alone. This indicates that while a sizeable component of the excess could be associated with interactions occurring outside of the TPC FV, a better fit is achieved when both events interacting inside and ones originating from outside the TPC FV are considered.

Figures 11 and 12 show the distributions of reconstructed shower energy and cosine of the reconstructed angle with respect to the beam direction for a subsample of the  $1\gamma$  signal events that contain one or more protons above the 35 MeV kinetic energy threshold ( $N_p$ ). In a complementary treatment to the  $1\gamma 0p$  ROI sample, the distributions are shown for shower energies binned from 0 to 600 MeV and the constraint channels used also have the one or more proton requirement. While the prediction is pulled down noticeably by the  $N_p$  constraining channels, the data still agrees well with the prediction within the uncertainties both before and after constraint, which can also be seen by the displayed goodness-of-fit information.

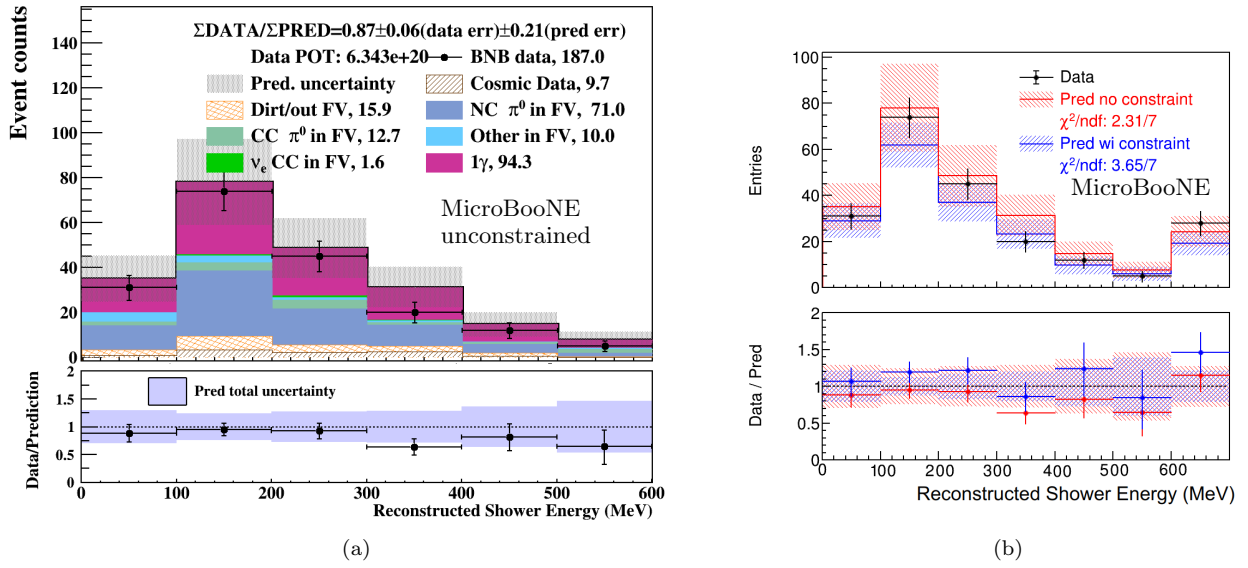

FIG. 11. (a): Shower energy for inclusive single-photon events with one or more protons (unconstrained). The signal is shown in solid pink. (b): Shower energy for inclusive single-photon selected events with one or more protons, before (red) and after (blue) constraint. The horizontal axis is reconstructed shower energy from 0 to 600 MeV with bin size of 100 MeV with the last bin as overflow.

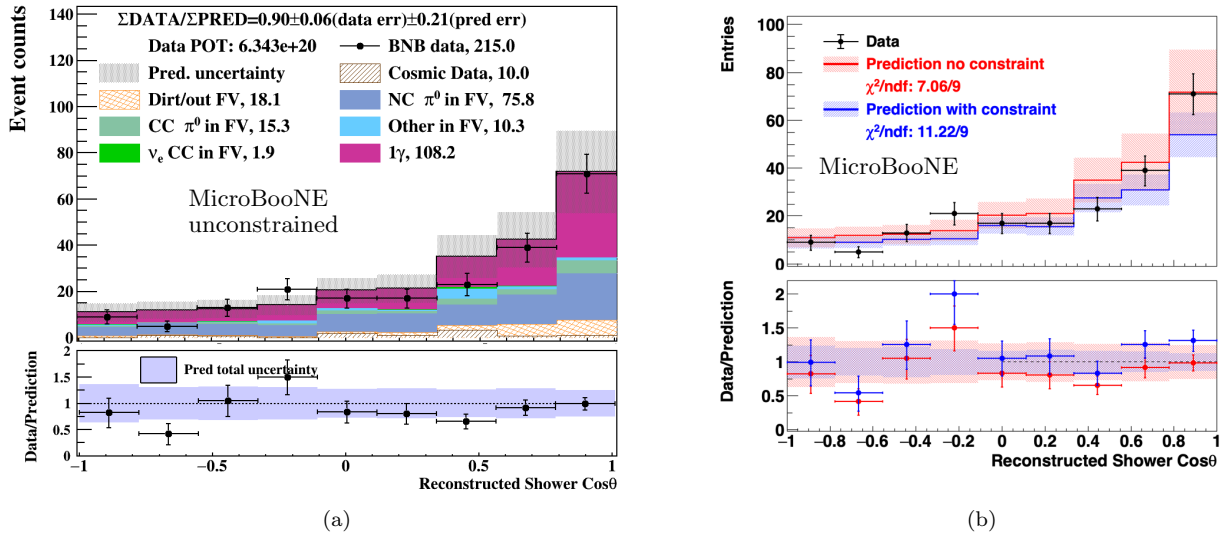

FIG. 12. (a): Cosine of reconstructed shower angle with respect to the beam for inclusive single-photon events with 1 or more protons (unconstrained). Signal is shown in solid pink. (b): Cosine of reconstructed shower angle with respect to the beam for single-photon selected events with 1 or more protons, before (red) and after (blue) constraint. The horizontal axis is reconstructed shower angle with bin size of  $\sim 0.22$ .

## VI. SHAPE FIT AND LEE MODEL

This section describes the statistical tests performed to investigate the origin of the excess events observed, as well as the empirical photon LEE model used to relate MicroBooNE's observation to MiniBooNE's excess.

Figure 13 shows the distribution of the  $\chi^2$ , calculated using the same Pearson formula used for the  $\chi^2/\text{n.d.f.}$  goodness-of-fit metrics used in this paper, for the data and 4 million pseudo-experiments generated from the constrained prediction in the 0 to 600 MeV shower energy distribution for the  $1\gamma 0p$  ROI. The resulting  $p$ -value of 0.03



and significance of  $2.2\sigma$  provides a “local significance” for this ROI.

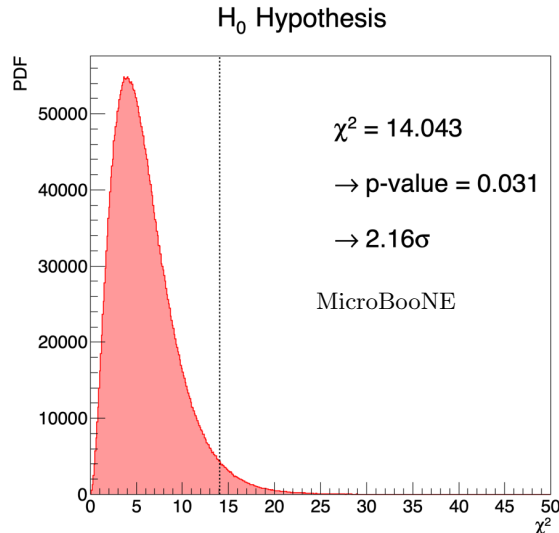

FIG. 13. Pearson  $\chi^2$  distribution for pseudo-experiments generated from the constrained shower energy distribution in the 0-600 MeV region for  $1\gamma 0p$  events. 4 million pseudo-experiments are used. The black dotted lines indicate the Pearson  $\chi^2$  value for the data.

Many theoretical models have been proposed to explain the MiniBooNE LEE. These include standard model backgrounds, light sterile neutrinos (and variations), heavy neutrino decay, and dark sectors, among others. These models have many valuable benefits: they allow interpretations of the LEE under a specific phenomenological hypothesis, and enable comparisons between the MiniBooNE and MicroBooNE data observations, provided the assumptions used in building these models are clearly stated. Any such model ultimately relies on assumptions on the interaction process that produces the observed excess events in the MiniBooNE detector. Yet, whatever model or interpretation is attributed to the LEE, it must ultimately be compatible with the kinematic observables which depend solely on the MiniBooNE detector’s efficiency at identifying and reconstructing electromagnetic showers: the energy and angle of the electromagnetic showers recorded in the detector. The model described here focuses on these fundamental detector observables. Given the null results of MicroBooNE’s first round of LEE searches, this model focuses on testing whether an excess of photon activity consistent with MiniBooNE’s observation is detected in MicroBooNE.

The model is constructed using the same procedure as the electron LEE model used in Ref. [2], but applied to photons instead. It relies on MiniBooNE’s simulation to evaluate the reconstruction efficiency and smearing of energy and angle for photons produced in the detector. The background subtracted MiniBooNE excess events of Ref. [3] are then unfolded into true space according to these efficiencies and smearing matrices with a 2D unfolding procedure in the shower kinematics. This procedure leads to an efficiency-corrected rate of photons as a function of true kinematics, which is the model’s hypothesis for the signal leading to the MiniBooNE excess.

This excess prediction in truth-space is next propagated to MicroBooNE. Doing so requires making several assumptions. We assume the excess events originate from the BNB flux, and therefore scale with the POT exposure of the detector and with the  $1/L^2$  distance of the detector from the target. Furthermore, predicting the rate of events in MicroBooNE requires an assumption on the interaction type. Three possible interaction types that could result in single-photon events are

1. A decay-induced interaction. The event rate for this assumption scales with the volume of the detector.
2. An interaction with target nucleons, which scales with the number of nucleons in the detector (“target mass”).
3. A coherent interaction, which scales as the number of target atoms.

All three are evaluated by this analysis. The predicted excess is then propagated through the MicroBooNE detector simulation and through the analysis selection, leading to a predicted spectrum of excess events observed in MicroBooNE under each hypothesis. The second hypothesis, scale by target mass, is the one shown in this paper.

Due to the assumption that no activity outside of the photon is present in the event, all comparisons are shown to the  $1\gamma 0p$  ROI results for this analysis. Figure 14 shows the distribution of selected  $1\gamma 0p$  events as a function of



shower angle, shower energy is shown in the main text. The LEE model prediction scaled by the target mass is shown in pink.

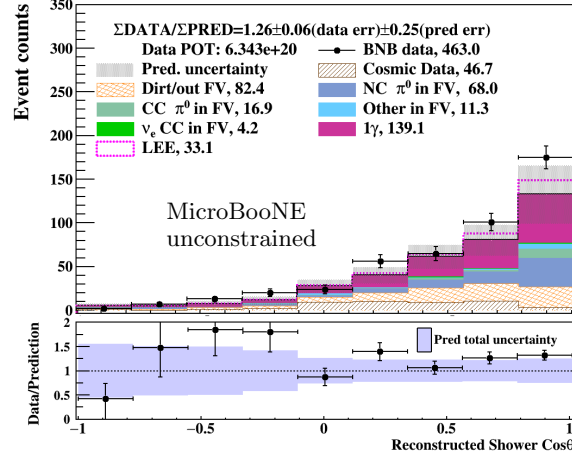

FIG. 14. Reconstructed shower angle for exclusive  $1\gamma 0p$  selected events, before constraint. The pink dotted line shows the MiniBooNE LEE model under the target nucleon interaction scaling assumption.

Figures 15 and 16 show the  $\Delta\chi^2$  test statistic constructed using the combined Neyman-Pearson (CNP) [4] method used to simultaneously compare the  $1\gamma 0p$  data sample to the constrained, nominal **GENIE** prediction ( $H_0$ ) and constrained, **GENIE** plus LEE- $\gamma$  model prediction ( $H_1$ ) for the shower energy and angle, respectively. Overall, we observe a larger data excess compared to the photon interpretation of the MiniBooNE LEE under the target nucleon interaction scaling assumption. When evaluated using the shower energy (angle), we show a slight preference for  $H_1$  over  $H_0$  with a  $p$ -value of 0.02 (0.01) for the  $H_0$  hypothesis and 0.14 (0.09) for the  $H_1$  hypothesis.

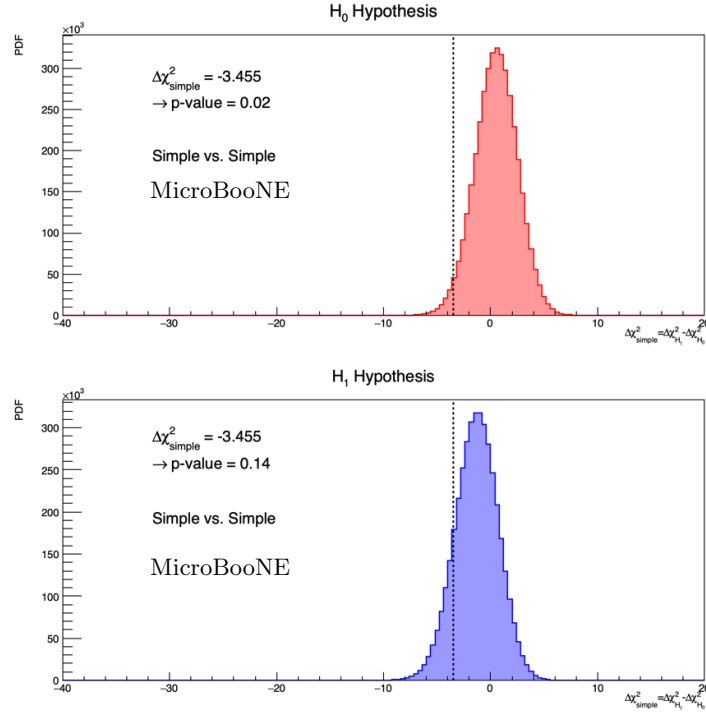

FIG. 15. MiniBooNE LEE model  $\Delta\chi^2$  for the full analysis, using the shower energy with range from 150-1250 MeV and the target nucleon interaction scaling assumption.

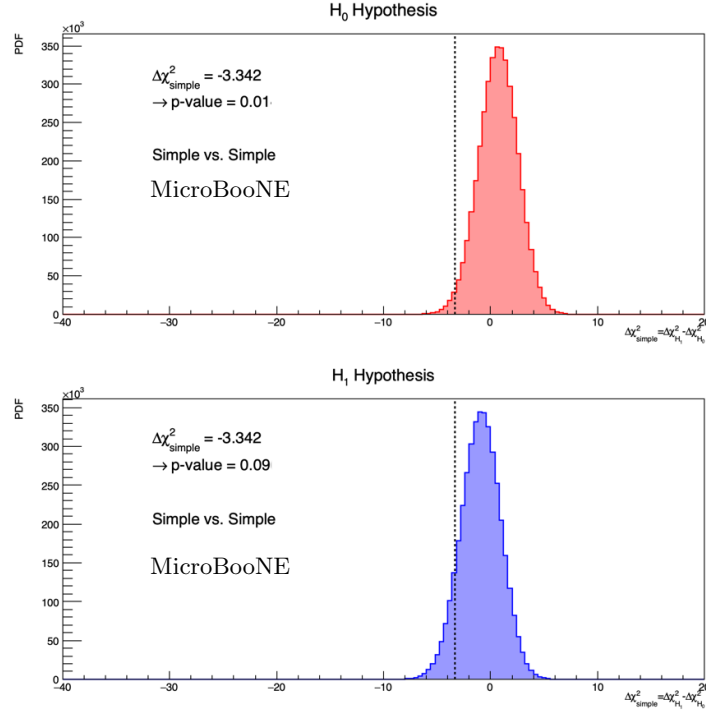

FIG. 16. MiniBooNE LEE model  $\Delta\chi^2$  for the full analysis, using cosine of the shower angle and the target nucleon interaction scaling assumption.

Figure 17 shows the shape-only fit to background-subtracted “excess” events discussed in the main text. The distribution shown here shows the results of all tested categories, which includes each of the five signal categories as well as the LEE model described above. Note that the LEE model has a sharp cut-off around 150 MeV, which affects the shape of the first two energy bins for this category in Figure 17.

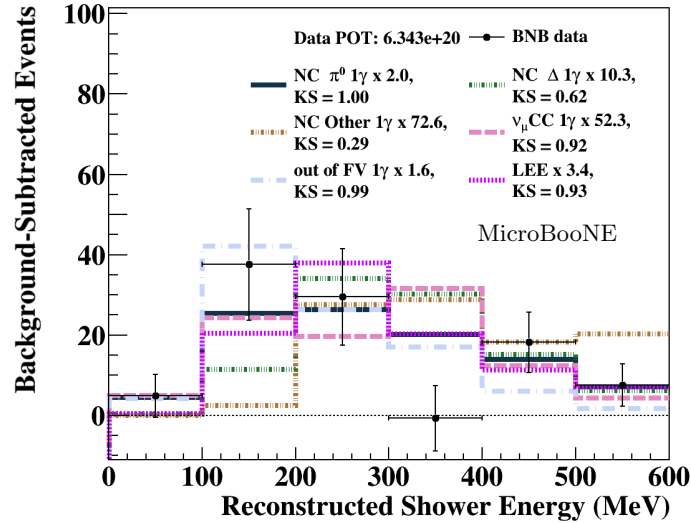

FIG. 17. Shape-only fit for  $1\gamma 0p$  background-subtracted “excess” events (data minus prediction). All single-photon signal event categories, as well as the LEE- $\gamma$  model, are shown alongside the best fit scaling parameter and the Kolmogorov-Smirnov test statistic. We do not apply a sideband constraint to the excess predictions. The error bars on the data points include both statistical and constrained systematic errors.

- 
- [1] P. Abratenko *et al.* (MicroBooNE Collaboration), Wire-cell 3D pattern recognition techniques for neutrino event reconstruction in large LArTPCs: algorithm description and quantitative evaluation with MicroBooNE simulation, J. Instrum. **17**, P01037 (2022).
  - [2] P. Abratenko *et al.* (MicroBooNE collaboration), Search for an Anomalous Production of Charged-Current  $\nu_e$  Interactions Without Visible Pions Across Multiple Kinematic Observables in MicroBooNE, arXiv e-prints (2024), arXiv:2412.14407 [hep-ex].
  - [3] A. A. Aguilar-Arevalo *et al.* (MiniBooNE Collaboration), Updated MiniBooNE neutrino oscillation results with increased data and new background studies, Phys. Rev. D **103**, 052002 (2021).
  - [4] X. Ji, W. Gu, X. Qian, H. Wei, and C. Zhang, Combined Neyman–Pearson chi-square: An improved approximation to the Poisson-likelihood chi-square, Nucl. Instrum. Meth. A **961**, 163677 (2020).
